# Supplementary material for: AlphaClean: Automatic Generation of Data Cleaning Pipelines
Source: arXiv:1904.11827 source file (2019-05-07)
Supplement: Supplementary file 1 [file appendix.tex]

\appendix
\label{s:appendix}

\section{Quality Functions}
Details about quality functions for exsiting stuff

\section{Data Transformations}

Details about data xforms that we used.

\section{Datasets}
\vspace{0.5em}\noindent\textbf{USCensus: } This dataset contains US Census records for adults and the goal is to predict  whether the adult earns more than $50,000$ dollars. It contains 32,561 records with 15 numerical and categorical attributes. This dataset contained missing values and coding inconsistencies.
Examples of data error include:
\begin{lstlisting}
#missing values
40,Private,121772,Assoc-voc,11,
Married-civ-spouse,Craft-repair,Husband, 
Asian-Pac-Islander,Male,0,0,40,(*\orange{\bf{?}}*),>50K

#coding inconsistency
57,Local-gov,110417,HS-grad,9,
Married-civ-spouse,Craft-repair,Husband,
White,Male,(*\orange{\bf{99999}}*),0,40,United-States,>50K
\end{lstlisting}

\vspace{0.5em}\noindent\textbf{Federal Election Commission Contributions: } The FEC provides a dataset of election contributions of 6,410,678 records with 18 numerical, categorical and string valued attributes. This dataset has a number of errors. There are missing values, formatting issues (where records have the wrong number of fields causing misaligment in parsing), and numerical outliers (negative contributions).

\begin{lstlisting}
#missing values
C00458844,"P60006723","Rubio, Marco","RUCINSKI,
ROBERT","APO","AE","090960009","US ARMY",
"PHYSICIAN",100,08-MAR-16,(*\orange{\bf{``''}}*),(*\orange{\bf{``''}}*),(*\orange{\bf{``''}}*),"SA17A",
"1082559","SA17.1074981","P2016"

#rejected contributions double recorded
C00458844,"P60006723","Rubio, Marco","SWAID, 
SWAID N. DR.","BIRMINGHAM","AL","352660827",
"NEWOLOGICAL SURGERY ASSOCIATES","PHYSICIAN",
(*\orange{\bf{-400}}*),28-DEC-15, "REDESIGNATION TO GENERAL","X",
"REDESIGNATION TO GENERAL","SA17A",
"1047126","SA17.892835B","P2016"
\end{lstlisting}
